# Supplementary material for: An Efficient Evolutionary Algorithm for Minimum Cost Submodular Cover
Source: arXiv:1908.01029 source file (2019-08-02)
Supplement: Supplementary file 1 [file appendix_pareto.tex]

\subsection{Pareto Optimization}
\label{appendix:pareto}

  Pareto Optimization Algorithms (POAs) are a type of EA for multi-objective optimization
  problems. In POAs, a notion of $\textit{domination}$ is defined on solutions.

In POAs, a notion of $\textit{domination}$ is defined on solutions. For MCSC domination is defined as
follows \cite{qian2015constrained}: $f(Y)\leq f(X)$ and $c(X)\leq c(Y)$ then $X$ weakly dominates $Y$.
$X$ dominates $Y$ if it weakly dominates $Y$ and at least one of the conditions are strict.
The population is a set of solutions where no solution dominates another. New solutions are generated by
random mutation of solutions in the population, and are added if no solution already in the population
dominates them. When a new solution is added, all solutions in the population that are dominated by the
new solution are removed from the population.
